# Supplementary material for: VLM-Guided Contact Retargeting and Generative Partner Modeling for Humanoid-Human Interaction
Source: arXiv:2610.28523 source file (2026-10-20)
Supplement: Supplementary file 1 [file 06-supp-NOT_USED.tex]

\section{VLM Contact Annotation: distance candidates and semantic verification}
\label{sec:supp:contact-annotation}

We annotate four contact-rich Inter-X actions: hug, pat-on-back, high-five, and link-arms.

\paragraph{Stage 1: distance candidates} We run SMPL-X forward kinematics on both bodies and, for every frame, group each person's arm mesh vertices by skinning weights into a \emph{hand} (wrist and fingers), \emph{forearm}, and \emph{upper-arm} region on each side. Each region's vertices are compared against every vertex of the partner mesh; pairs within $15\,\text{cm}$ are grouped by (contacting arm region, contacted SMPL-X joint), the closest pair is retained per group, and consecutive frames are merged into events lasting at least $0.5\,\text{s}$. Each event records its time window, the contacting region, the contacted partner joint, the closest actor- and partner-side vertices, and the minimum and average mesh-to-mesh distances.

\paragraph{Stage 2: VLM verification} Each event is verified against the corresponding video by a vision-language model (Gemini~2.0 Flash). We render the SMPL-X motion from three camera viewpoints, concatenate the views horizontally, sample at $5\,\text{fps}$, and split the video into $1\,\text{s}$ chunks; each chunk is sent with the action label and a textual description of every event that overlaps it. The VLM is prompted to first list the contact patterns expected for the action (e.g., palm-to-palm for high-five, palm-to-back and forearm-to-shoulder for hug) and then to assign each event one of four semantic labels (\emph{essential}, \emph{incidental}, \emph{unnecessary}, or \emph{avoid}), together with the contacting and contacted surfaces (palm/inner vs.\ back/outer) and the views in which the contact is visible with high confidence. Only events labelled essential or incidental survive.

\paragraph{Output} For each of the six contact sites (left or right \emph{hand}, \emph{forearm}, \emph{upper-arm}) and every timestep $t$, the annotation provides a binary contact flag, the closest vertex on the actor mesh, the contacted target vertex on the partner mesh, and the name of the contacted SMPL-X joint. The contact reward of Eq.~\ref{eq:contact-reward} and the Stage~2 contact co-optimisation in retargeting consume the hand-region subset of these flags via the wrist body and palm site.


\section{Contact Reward: coefficients and force gate}
\label{sec:supp:contact-reward}

The per-hand contact reward of Eq.~\ref{eq:contact-reward} in the main text is instantiated with positive coefficient $\alpha = 0.5$, exponential distance decay $\kappa = 3.0\,\text{m}^{-1}$, contact-off penalty coefficient $\beta = 0.01$, and force gate $\phi(F) = \min\!\big(\exp(F - \tau),\, 1\big)$ with threshold $\tau = 1\,\text{N}$. The per-step reward is the sum over the two wrists, $r_t = \sum_h r^h_t$. We weight the contact reward at $w_{\text{contact}} = 10$ in the aggregate teacher and student reward so that the contact term dominates the wrist-tracking error on labelled frames.

The palm offset in the wrist link frame is $\mathbf{o}_{\text{palm}} = (0.08, 0, 0)\,\text{m}$ for both hands, matching the palm site of the Unitree G1 MJCF. The targeted partner joint is one of the SMPL-X body, hand, or face joints indicated by the per-frame VLM annotation; the world-frame target position $\mathbf{q}^h_t$ is read from the same SMPL-X kinematics that drives the visual mesh of Sec.~\ref{sec:supp:rendering}.

The reward exports two binary masks $m^L_t, m^R_t$ marking the per-environment contact-labelled state of each wrist. These masks gate the wrist and elbow components of the relative-frame body-position and body-velocity tracking rewards: on labelled frames the corresponding rows of the tracking error are zeroed so the arm chain has the kinematic freedom to reach the contact target.


\section{Teacher Policy: observation breakdown, reward weights, and training}
\label{sec:supp:teacher}

\paragraph{Observation} The teacher's proprioception vector is the 108-dimensional concatenation $\mathbf{o}^{\text{prop}}_t = [\boldsymbol{\omega}_b,\, \mathbf{g}_b,\, \mathbf{q},\, \dot{\mathbf{q}},\, \mathbf{p}^{\text{ee}}_b,\, \mathbf{a}_{t-1}]$, with components base angular velocity (3), projected gravity (3), 29 joint positions, 29 joint velocities, five end-effector positions in the base frame (15), and the previous action (29). The privileged motion command and the partner state are passed in their full per-frame form (target G1 joint targets, target root pose, target key body positions/orientations, contact label and target-joint index, partner root and body positions relative to the robot base). Small per-term observation noise (joint positions $\sigma{=}0.01$, joint velocities $\sigma{=}0.5$, base angular velocity $\sigma{=}0.2$, partner positions $\sigma{=}0.1$) regularises the policy during rollouts; the critic receives the same terms without noise.

\paragraph{Action} The teacher emits $\mathbf{a}_t \in \mathbb{R}^{18}$: four HOMIE locomotion commands $(v_x, v_y, \omega_z, h)$ and 14 residual upper-body joint offsets. The HOMIE tracker selects between a walk MLP and a stand MLP based on a command-norm threshold of $0.1$ and converts the 4-d command into 15 lower-body joint actions. The 14 residuals are added in action space to the demonstration's reference arm pose. Both the walk and stand sub-policies are kept frozen throughout teacher training.

\paragraph{Reward weights} The aggregate per-step reward is
\[
  r_t = 10\,r^{\text{contact}}_t + 0.5\,r^{\text{root\,pos}}_t + 0.5\,r^{\text{root\,ori}}_t + r^{\text{body\,pos}}_t + r^{\text{body\,ori}}_t + r^{\text{body\,vel}}_t + r^{\text{body\,ang}}_t + r^{\text{no\,fly}}_t + r^{\text{reg}}_t,
\]
with relative-frame body-position $\sigma = 0.3\,\text{m}$, body-orientation $\sigma = 0.4\,\text{rad}$, body-velocity $\sigma = 1.0\,\text{m/s}$, body-angular-velocity $\sigma = 3.14\,\text{rad/s}$, and the wrist/elbow rows of the body terms masked on contact-labelled frames. Regularisation: action rate $-3{\times}10^{-2}$, joint velocity $-2{\times}10^{-4}$, joint acceleration $-1{\times}10^{-7}$, torque $-1{\times}10^{-4}$, DOF-position soft limit $-100$ (with $0.9$ soft-limit ratio), DOF-velocity soft limit $-1{\times}10^{-3}$, torque soft limit $-3{\times}10^{-2}$. The no-fly term rewards at least one foot in contact ($+1$ when satisfied).

\paragraph{Initialisation} Episodes use a hybrid \textit{physical state initialisation}: with probability $0.5$ the episode restarts from the policy's own recent on-policy state; otherwise it is seeded from the demonstration's reference frame perturbed by Gaussian noise with joint positions $\sigma = 0.1$, root translation $\sigma_{xyz} = (0.05, 0.05, 0.01)\,\text{m}$, root orientation $\sigma = (0.1, 0.1, 0.2)\,\text{rad}$, root linear velocity $\sigma = (0.5, 0.5, 0.2)\,\text{m/s}$, and root angular velocity $\sigma = (0.52, 0.52, 0.78)\,\text{rad/s}$. The initial action noise std is $\sigma_{\text{init}} = 0.5$. The partner is replayed kinematically with gravity disabled and a reference PD controller; robot--partner collisions are enabled.

\paragraph{PPO} Both actor and critic are 3-layer MLPs with hidden sizes $[512, 256, 128]$ and ELU activations. We use PPO~\cite{schulman2017ppo} with $\gamma = 0.99$, GAE $\lambda = 0.95$, clipping $0.2$, 8 update epochs per rollout, 4 minibatches, entropy coefficient $0.01$, and AdamW with learning rate $10^{-5}$ for both actor and critic. We collect 24 environment steps per iteration across 4{,}096 parallel Isaac Sim environments on a single L40S GPU.

\section{Retargeting User Study: protocol and per-question results}
\label{sec:supp:retarget-userstudy}

\paragraph{Protocol} For each of $80$ held-out human--human interaction
sequences we render the four retarget conditions of Table~\ref{tab:retarget}
(GMR, OmniRetarget, Ours w/o VLM contact annotation, Ours) side-by-side
together with the original SMPL-X demonstration as a $3$-view orbit
reference at the top of the screen. The four method panels are randomly
assigned to the on-screen positions $A,B,C,D$ per trial. For every trial
the participant provides three independent rankings (rank~$1$ = best,
rank~$4$ = worst, no ties): (Q1) \emph{G1 contact $+$ motion quality},
(Q2) \emph{Human contact $+$ motion quality}, (Q3) \emph{Overall
preference}. Participants were instructed to weight pose consistency with
the demonstration, contact-location accuracy with respect to the action
label, jitter, mesh penetration, and joint-pose stability (over-stretched
limbs / hyperextension) together, and to prefer a refined-but-cleaner
result over a faithful reproduction of any noise present in the original.
Sequence order is per-participant random (deterministic from a hash of
the participant name so that resumed sessions stay reproducible).

\paragraph{Results} We collect $N{=}8$ participants who finished all
$80$ trials with valid $\{1,2,3,4\}$ permutations on all three questions
(median active time per participant $\approx 2.6\,$h). For each
participant we compute the mean rank of each condition averaged over the
$80$ sequences; Table~\ref{tab:supp-userstudy} then reports the
across-participant mean $\pm$ standard error (SEM, $n{=}8$) per
(question, condition) pair.

\begin{table}[h]
  \centering
  \small
  \caption{\textbf{User study: per-question mean ranks $\pm$ SEM
  ($n{=}8$ participants, $80$ sequences each, lower is better).}
  Each entry is the across-participant mean of per-participant
  per-condition mean ranks. Ranks lie in $\{1,2,3,4\}$ with
  $1{=}\text{best}$.}
  \label{tab:supp-userstudy}
  \begin{tabular}{lccc}
    \toprule
    Method & Q1: G1 contact & Q2: Human contact & Q3: Overall \\
           & + motion\,$\downarrow$ & + motion\,$\downarrow$ & preference\,$\downarrow$ \\
    \midrule
    GMR                                 & $3.67 \pm 0.06$ & $3.55 \pm 0.06$ & $3.68 \pm 0.05$ \\
    OmniRetarget                        & $2.58 \pm 0.08$ & $2.44 \pm 0.09$ & $2.52 \pm 0.08$ \\
    \midrule
    Ours w/o VLM contact annotation     & $1.99 \pm 0.07$ & $2.15 \pm 0.08$ & $2.04 \pm 0.08$ \\
    \rowcolor{LightGreen}
    Ours                                & $\textbf{1.76} \pm 0.04$ & $\textbf{1.85} \pm 0.04$ & $\textbf{1.77} \pm 0.04$ \\
    \bottomrule
  \end{tabular}
\end{table}

The full pipeline takes the best mean rank on every question. The
largest gap on Q1 (G1 contact: $1.76$ vs.\ OmniRetarget's $2.58$, a
$0.82$-rank improvement) confirms that the VLM-guided contact annotation
is the component most directly tied to robot-side contact correctness.
Removing the VLM annotation (\emph{Ours w/o VLM}) costs about $0.23$
rank on Q1 and $0.27$ on Q3, consistent with the precision drop reported
in Table~\ref{tab:retarget}. GMR is ranked last on every question across
participants ($\geq 3.55$), reflecting its lack of any contact-aware
objective.


\section{Photorealistic Human Rendering: sensor and pipeline}
\label{sec:supp:rendering}

\paragraph{Depth sensor} We simulate an Intel RealSense D435 mounted on the G1 torso, matching the VisualMimic~\cite{ze2025visualmimic} mount frame (\texttt{d435\_link}: offset $[0.058, 0.018, 0.430]\,\text{m}$ from the torso link, approximately $46^{\circ}$ pitch-down). The camera renders at $30\,\text{Hz}$ with $87^{\circ}$ horizontal field of view and $3\,\text{m}$ far clip; raw depth is clipped at the far clip and consumed at the native render resolution. Configuration \texttt{v6} (used for the student of Sec.~\ref{sec:supp:student}) renders at $192{\times}108$ without down-sampling and supplies a 5-frame temporal stack at $25$ control-step intervals (i.e., $\{0, 0.5, 1.0, 1.5, 2.0\}\,\text{s}$ at $50\,\text{Hz}$ control). These intrinsics match those of the physical D435 we deploy on the real robot.

\paragraph{SMPL-X visual mesh} For each parallel environment we create a single visual-only \texttt{UsdGeom.Mesh} of the SMPL-X body topology ($10{,}475$ vertices, $20{,}908$ triangles, double-sided, semi-transparent neutral material) parented under the partner prim. The recipient's collision capsules are hidden from the depth camera but remain in the physics scene. At every control step we read each environment's current motion frame, batch the per-environment SMPL-X parameters (shape $\boldsymbol{\beta}\in\mathbb{R}^{10}$, global orientation $\in\mathbb{R}^3$, body pose $\in\mathbb{R}^{63}$, per-hand pose $\in\mathbb{R}^{45}$, root translation $\in\mathbb{R}^3$) into a single GPU forward pass through the SMPL-X model, and write the resulting vertex positions back to each USD mesh. Source-FPS to control-FPS resampling ($50\,\text{Hz}$ control) is handled per environment so each scene reads the correct demonstration frame even under randomised start offsets and per-environment speed warping.

\paragraph{FOV-filtered training split} A torso-mounted, $87^{\circ}$-HFOV camera cannot see a partner who is, in the demonstration, immediately beside or behind the humanoid. We pre-filter the training corpus to clips in which the recipient remains within the camera frustum for the entire horizon (denoted \texttt{group-split-train-fov-person}); evaluation uses the corresponding held-out FOV-filtered split. Demonstration clips are additionally truncated to $10\,\text{s}$ to bound rollout memory.


\section{Depth-based Student Policy: architecture, losses, and distillation}
\label{sec:supp:student}

\paragraph{Observations} At every control step the student receives (i) a 5-frame temporal stack of egocentric $192{\times}108$ depth images at offsets $\{0, 0.5, 1.0, 1.5, 2.0\}\,\text{s}$ in the past, (ii) a 5-step short-term proprioception history ($5 \times 108 = 540$ dims; same composition as the teacher's $\mathbf{o}^{\text{prop}}$), and (iii) a $200$-step ($4\,\text{s}$ at $50\,\text{Hz}$) long-term proprioception history. No partner pose, motion command, contact label, or camera-pose state is exposed at inference.

\paragraph{Depth backbone} A shared depth CNN with the VisualMimic~\cite{ze2025visualmimic} backbone embeds each depth frame independently: $\text{Conv}_{5{\times}5}{:}1{\to}16 \to \text{ELU} \to \text{MaxPool}_{2} \to \text{Conv}_{3{\times}3}{:}16{\to}32 \to \text{ELU} \to \text{MaxPool}_{2} \to \text{Conv}_{3{\times}3}{:}32{\to}64 \to \text{ELU} \to \text{MaxPool}_{2} \to \text{Linear}{\to}256 \to \text{Linear}{\to}64$. Concatenating the five 64-d frame embeddings gives a 320-d temporal depth representation.

\paragraph{Long-term proprio encoder} A 1D-CNN (kernel $5$, stride $2$ for the first two layers, then $3,3$; channels $108{\to}128{\to}128{\to}128{\to}64$, ELU after each, adaptive average pool, $\text{Linear}{\to}128$) maps the 200-step proprioception window to a 128-d embedding. This replaces the camera-pose history that contact anticipation would otherwise require but that is unavailable on hardware.

\paragraph{Conditional VAE} Let $\mathbf{c}_t$ be the concatenation of the temporal depth embedding (320), short-term proprio history (540), and long-term proprio embedding (128). The \textit{prior} maps $\mathbf{c}_t$ through a $[512, 512, 256, 128]$ MLP to a diagonal Gaussian $\mathcal{N}(\boldsymbol{\mu}_p, \boldsymbol{\sigma}_p^2)$ with latent dimension $64$. The \textit{encoder} (training only) maps the privileged motion command $\mathbf{o}^{\text{mc}}_t$ ($232$ dims) through a matched $[512, 512, 256, 128]$ MLP to $\mathcal{N}(\boldsymbol{\mu}_e, \boldsymbol{\sigma}_e^2)$. We combine the two heads residually, $\boldsymbol{\mu}_z = \boldsymbol{\mu}_p + \boldsymbol{\mu}_e$, and pass $[\mathbf{c}_t, \mathbf{z}_t]$ through a $[512, 512, 512, 256, 128]$ trunk MLP that emits the same 18-dim HOMIE-plus-arm action mean as the teacher. All MLPs use ELU activations. At deployment, $\mathbf{z}_t = \boldsymbol{\mu}_p$.

\paragraph{Pose-anticipation auxiliary head} A DDPM denoiser conditioned on the prior trunk features predicts past, current, and short-horizon future human and G1 state. Targets cover the 5 past/current frames at $\{0, 0.5, 1.0, 1.5, 2.0\}\,\text{s}$ and 3 future frames at $\{0.5, 1.0, 1.5\}\,\text{s}$ ahead, with per-frame dimensions $60{+}60{+}3{+}120$ (positions, linear velocities, root velocity, 6D rotations) for the 20 SMPL-X key bodies. The G1 future head additionally predicts root state (4), end-effector positions (15) and velocities (15), and joint positions (29) and velocities (29) for each of the 3 future frames ($92 \times 3$). The denoiser is a 3-layer MLP with hidden width $1024$ and SiLU activations, a cosine $T=20$ noise schedule, sinusoidal timestep embedding, and EMA-normalised targets. We use a fixed initial DDIM noise per environment to keep predictions temporally consistent across control steps, and an $80\%$/$20\%$ split between a GENMO-style single-step pose-estimation loss (coefficient $\lambda_{\text{est}} = 1.0$) and a multi-step DDIM forward-prediction loss (coefficient $\lambda_{\text{pose}} = 0.5$). Per-frame losses are gated by the fraction of pixels covered by the partner mesh: frames with less than $30\%$ human coverage contribute neither gradient nor running-statistics updates.

\paragraph{Distillation loss} The full loss of Eq.~\ref{eq:student-loss} in the main text combines an L2 behaviour-cloning term against the teacher action (after converting the teacher's residual arm actions to absolute via the demonstration's reference arm pose), the conditional-VAE KL between the privileged encoder posterior and the deployable prior, and the two pose objectives above. We use on-policy DAgger with mixing coefficient $\beta = 0$ from the first epoch: rollouts are pure student trajectories and the teacher acts only as a per-state supervisor.

\paragraph{Training infrastructure} We train the student on 128 parallel Isaac Sim environments on a single L40S GPU (limited by depth-rendering throughput), with the partner replayed kinematically and the photorealistic SMPL-X mesh of Sec.~\ref{sec:supp:rendering} active. The student is initialised with $\sigma_{\text{init}} = 0.01$ action noise on top of the demonstration's physical state. Demonstration-time augmentation includes speed warping $[0.8, 1.2]\times$, start-offset jitter up to $1\,\text{s}$, G1 spatial-offset jitter of $0.2\,\text{m}$ and yaw jitter up to $\pi/4$. Depth-image augmentation applies random pixel dropout and additive noise with statistics matching the deployed D435; the deepest pixels are clamped to the $3\,\text{m}$ far clip. Periodic evaluation every $500$ iterations on the held-out FOV-filtered split selects the deployable checkpoint.


\section{Generative Partner-State Modeling: generative vs.\ deterministic prediction head}
\label{sec:supp:gen-vs-det}

We learn partner-state prediction with a generative (diffusion-based) objective rather than a deterministic regressor because, under close-contact interaction, the partner is rarely fully observable: large body regions are occluded or leave the camera field of view, so many partner configurations are consistent with the same egocentric depth and partner-state inference is inherently multimodal. A deterministic head regressing a single target under an L2 loss collapses this distribution onto its mean, an averaged prediction that lies between the plausible modes and need not be a valid pose. The diffusion-based head instead models the full conditional distribution, keeping the deployable observation embedding $\mathbf{c}_t$ aligned with interaction-relevant structure that mean-seeking regression discards.

We test this directly. \emph{Ours (deterministic)} replaces the diffusion-based head of Sec.~\ref{sec:supp:student} with a same-capacity MLP that regresses the identical past, present, and future targets under an L2 loss; everything else (depth backbone, conditional VAE, contact reward, augmentation, single-step $\mathcal{L}_{\text{pose}}$) is unchanged. \emph{Ours (generative)} is our diffusion-based head ($\mathcal{L}_{\text{gen}}$ in Eq.~\ref{eq:student-loss}), reproducing the \emph{Ours} row of Table~\ref{tab:student}.

\begin{table}[h]
  \centering
  \small
  \caption{\textbf{Generative vs.\ deterministic partner-state prediction.}
  Student contact recall (\%) on the held-out evaluation split. Both
  variants share the depth student of Sec.~\ref{sec:supp:student} and
  differ only in the partner-state prediction head: a direct-regression
  MLP under an L2 loss (deterministic) or the diffusion-based head
  (generative).}
  \label{tab:supp-gen-vs-det}
  \begin{tabular}{lccccc}
    \toprule
    Method & Hug & Shake-hand & Pat-on-back & link-arm & high-five \\
    \midrule
    Ours (deterministic) & \tbd{} & \tbd{} & \tbd{} & \tbd{} & \tbd{} \\
    \rowcolor{LightGreen}
    Ours (generative)    & 38.0 & 78.6 & 23.8 & 30.1 & 15.3 \\
    \bottomrule
  \end{tabular}
\end{table}

Table~\ref{tab:supp-gen-vs-det} shows that the generative head improves held-out contact recall over the deterministic regressor across interactions, widest where the partner is most often occluded, confirming that latent partner-state inference under severe partial observability is better served by a distribution-modelling objective than by mean-seeking regression.
